# Supplementary material for: Percolation transition in entangled granular networks
Source: arXiv:2509.00216 ancillary file (2025-09-03)
Supplement: Supplementary file 1 [file Supplementary_Information.pdf]

# Supplementary Information for “Percolation transition in entangled granular networks”

Seongmin Kim, Daihui Wu, and Yilong Han  
*Department of Physics, The Hong Kong University of Science and Technology, Hong Kong, China*

(Dated: September 3, 2025)

## SUPPLEMENTARY FIGURE: RING CONTINUUM PERCOLATION MODEL

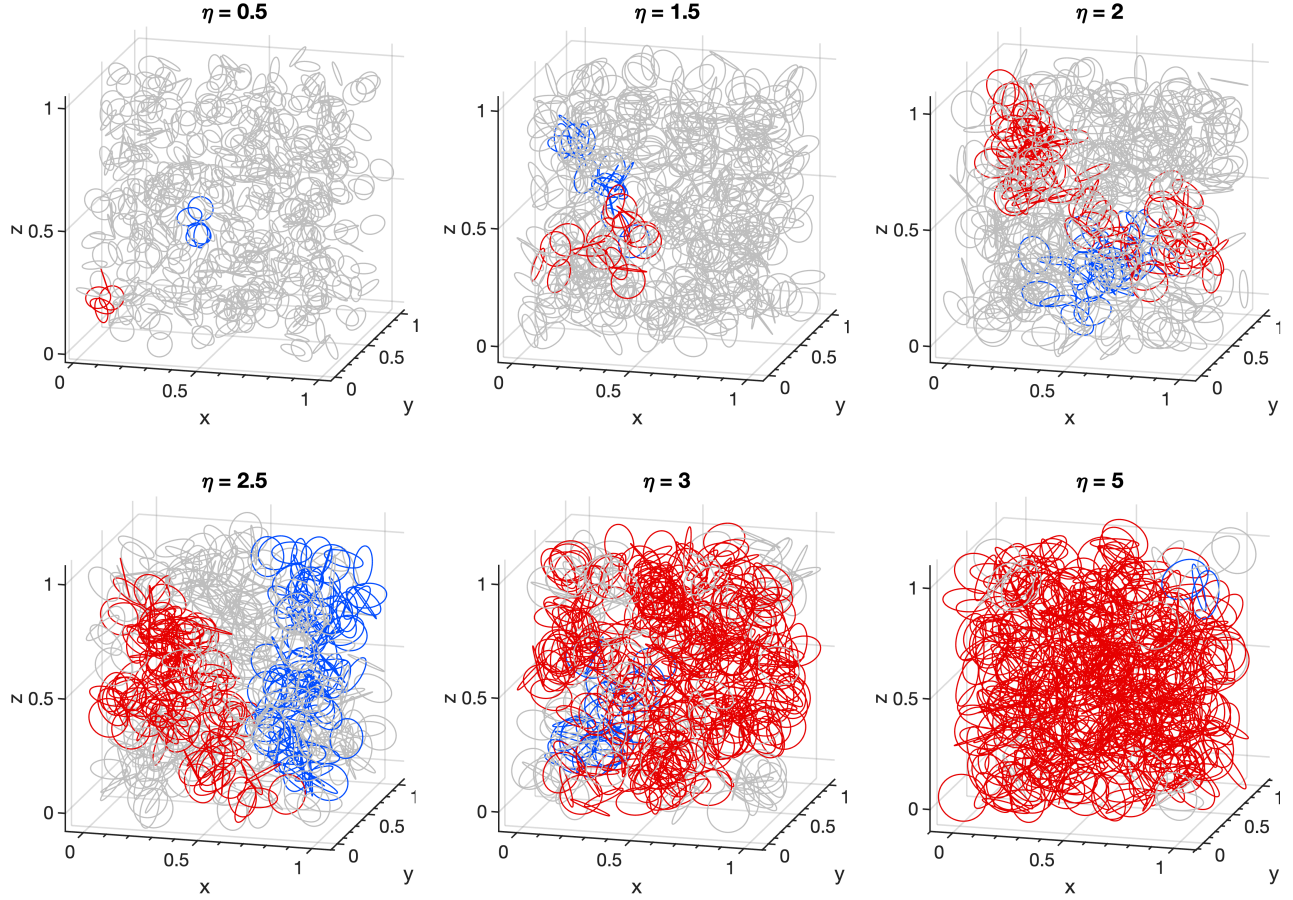

Supplementary Figure S1: Snapshots from Monte Carlo simulation of the CP model for  $N = 500$  rings at different reduced densities,  $\eta \equiv nv_{\text{ex}}^{\text{ring}} = n\pi D^3/3$ . Red rings represent the largest cluster. Blue rings represent the second largest cluster. The largest cluster becomes giant (i.e., percolating) at  $\eta \gtrsim 2.5$ , while the second largest cluster size peaks near  $\eta = 2.5$ , which is consistent with the  $S_1(\eta)$  and  $S_2(\eta)$  curves for  $N = 500$  in Extended Data Fig. 7a,b.

## SUPPLEMENTARY DISCUSSION: ADJACENCY SPECTRA OF NETWORKS

An  $N$ -node network can be described by an  $N \times N$  adjacency matrix  $\mathbf{A} = (A_{ij})$ .  $A_{ij} = 1$  if node  $i$  is connected to node  $j$ ; otherwise  $A_{ij} = 0$ . For our undirected network,  $\mathbf{A}$  is symmetric, and thus all its  $N$  eigenvalues  $\lambda_i$  are real. The distribution of these eigenvalues, i.e., the adjacency spectrum  $P(\lambda)$ , reflects the topological properties of the network [S1]. We compare the adjacency spectra of the lifted C-particle networks, ER random networks, and networks from the sphere CP and ring CP models (Extended Data Fig. 9).

In graph theory, discrete peaks of  $P(\lambda)$  at  $-1$  and  $0$  indicate redundant “symmetric motifs”, subsets of nodes that

share the same neighbors [S2, S3]. A symmetric pair of nodes that share the same neighbors generates an eigenvalue of  $-1$  when they are connected (Extended Data Fig. 9m), and an eigenvalue of  $0$  when they are not connected (Extended Data Fig. 9n). An eigenvalue of  $0$  can also be generated when the neighbors of a node are shared by multiple nodes that are disconnected from each other (Extended Data Fig. 9o). Furthermore, a non-negligible fraction of triangles produce a positively skewed spectrum as well as a  $-1$  peak [S4].

Comparing the peaks and skewness in Extended Data Fig. 9 reveals that the spectra of C-particle networks are similar to those of spatial network models, especially the ring CP model. For instance, at  $\langle k \rangle = 3.3$  and  $5.7$ , both C-particles and ring CP models show positively skewed spectra with two clear peaks at  $-1$  and  $0$ , and these peaks are also visible in their largest clusters (orange area in Extended Data Fig. 9b,c). The sphere CP model also has positively skewed spectra, but with a smaller peak at  $0$  that is not even present in the largest cluster (Extended Data Fig. 9h,i). These spatial networks differ markedly from ER random networks, which lack node positions and have unskewed spectra with a vanishing peak at  $-1$  (Extended Data Fig. 9k,l). In short, the adjacency spectra of C-particle networks are similar to those of the ring CP model and lie between those of the sphere CP model and ER random networks in terms of peak height and skewness.

The presence of the  $-1$  peak and positive skewness in the C-particle spectra indicates a significant number of triangles due to the position-dependent nature of entanglement. Only particles within a certain distance can be entangled, thus forming more connected symmetric motifs compared with ER random networks. In addition, the peak at  $0$  is higher in C-particle networks (Extended Data Fig. 9b,c) than in the sphere CP model (Extended Data Fig. 9h,i), suggesting that the former have more disconnected symmetric motifs due to the orientation-dependent nature of entanglement. In the sphere CP model, two spheres are connected when their distance is less than one diameter. By contrast, in the ring CP model and C-particle systems, two circles are connected only when both their distance and orientations are within a certain range. This anisotropic connection results in a less clustered structure, where the symmetric nodes are less connected than in the sphere CP model.

#### SUPPLEMENTARY METHODS: CONTACT MODEL FOR DEM SIMULATION

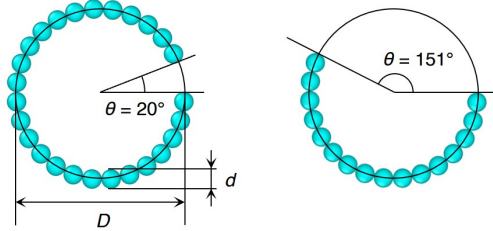

Supplementary Figure S2: Particle shape used in DEM simulations.

| $\theta$                               | 20.0°  | 33.1°  | 46.1°  | 59.2°  | 72.3°  | 98.5°  | 111.5° | 124.6° | 137.7° | 150.8° |
|----------------------------------------|--------|--------|--------|--------|--------|--------|--------|--------|--------|--------|
| Particle mass ( $m$ )                  | 26     | 25     | 24     | 23     | 22     | 20     | 19     | 18     | 17     | 16     |
| Normal elastic constant ( $k_n$ )      | $10^6$ | $10^6$ | $10^6$ | $10^6$ | $10^6$ | $10^6$ | $10^6$ | $10^6$ | $10^6$ | $10^6$ |
| Damping constant ( $\gamma_n$ )        | 120    | 120    | 120    | 120    | 120    | 120    | 120    | 120    | 120    | 120    |
| Restitution coefficient ( $\epsilon$ ) | 0.499  | 0.506  | 0.513  | 0.521  | 0.528  | 0.545  | 0.554  | 0.563  | 0.572  | 0.582  |
| Friction coefficient ( $\mu_p$ )       | 0.4    | 0.4    | 0.4    | 0.4    | 0.4    | 0.4    | 0.4    | 0.4    | 0.4    | 0.4    |

Supplementary Table S1: Particle properties used in the DEM simulations. Particle mass, elastic constant, and damping constant are in arbitrary units. Restitution coefficient and friction coefficient are dimensionless.

We perform DEM simulations on C-shaped granular particles using LAMMPS (Large-scale Atomic/Molecular Massively Parallel Simulator) [S5]. Specifically, a C-particle with the smallest opening angle  $\theta = 20^\circ$  is modeled by 26 small spherical particles with a diameter of  $d = 1$ , resulting in a centerline diameter  $D = 8.782$  (Supplementary Figure S2). This diameter-to-thickness ratio is similar to that of C-particles in the experiment. Larger openings are achieved by removing the small spherical particles. The contact forces between granular particles are modelled by

the standard spring-dashpot model capped by Coulomb friction [S6]: the normal force  $F_n = k_n \delta_n - m_{\text{eff}} \gamma_n v_n$  and the tangential force  $F_t = k_t \delta_t$  where  $\delta_n$  and  $\delta_t$  are the normal and tangential components of the contact displacement.  $v_n$  is the normal component of the relative velocity. The normal elastic constant  $k_n$  is set to be large enough to support the weight of 4000 particles with a single contact while keeping  $\delta_n$  less than 1.2% of  $D$ . The tangential elastic constant  $k_t$  is set as  $\frac{2}{7}k_n$ . The restitution coefficient of the binary head-on collision can be estimated as

$$\epsilon = \exp \left[ -\pi \left( \frac{4k_n}{m_{\text{eff}} \gamma_n^2} - 1 \right)^{-\frac{1}{2}} \right] \quad (1)$$

[S7–S9], where  $m_{\text{eff}}$  is the effective mass which becomes half the C-particle mass ( $m/2$ ) in our case. Since we use fixed  $k_n$ ,  $\gamma_n$ , and mass density, the restitution coefficient varies from 0.5 to 0.58 as  $\theta$  changes, but the choice of  $\epsilon$  is known to have minimal effect on the macroscopic mechanical behavior of dense hard particles [S7, S10, S11]. The exact particle properties are shown in Supplementary Table S1.

We convert unitless simulation time to real time to match the experiment. In the simulation, the gravitational acceleration  $g$  and the mass of the small spherical particles are both set to 1. Because the simulation uses arbitrary units, the resulting simulation time  $t_{\text{sim}}$  is unitless and must be converted to real time  $t_{\text{real}}$  to match the experiment. To achieve this, we set the characteristic time  $\sqrt{2D/g}$  to be the same in the simulation and the experiment. This time represents how long it takes for a particle to free fall a distance equal to its diameter  $D$  under gravity. Then,  $t_{\text{real}}$  can be calculated from  $t_{\text{sim}}$  as follows:

$$t_{\text{real}} = t_{\text{sim}} \frac{\sqrt{D_{\text{real}}/g_{\text{real}}}}{\sqrt{D_{\text{sim}}/g_{\text{sim}}}} = t_{\text{sim}} \times 1.022 \times 10^{-2} \text{ s}. \quad (2)$$

The simulation time step is set to be less than 4.5% of the binary head-on collision time,  $\tau_c = \pi \sqrt{\frac{m_{\text{eff}}}{k_n} (1 + (\ln \epsilon / \pi)^2)}$ , which is derived from a half period of damped oscillation.

## SUPPLEMENTARY VIDEOS

**Supplementary Video 1: Sample preparation process in the experiment.** Entangled C-particles ( $\theta = 25^\circ$ ) become disentangled as they trickle through the top vibrating funnel to the bottom funnel at rest. The disentangled C-particles in the bottom funnel will be used in the vibration-induced cluster formation measurement. The vibration frequency  $f = 20$  Hz and amplitude  $A = 1.55$  mm such that the peak acceleration is  $A(2\pi f)^2 = 2.5g$  ( $g = 9.8$  m/s<sup>2</sup>).

**Supplementary Video 2: Lifting clusters after four different vibration durations in the experiment.** Entangled clusters of C-particles ( $\theta = 25^\circ$ ) are lifted and weighed after being vibrated for  $t = 4$  s (3–15 s in the video), 8 s (15–28 s), 15 s (28–38 s), and 120 s (38–46 s). The weight in grams is shown on the blue screen. At  $t = 4$  s, there are many small clusters without a giant cluster. At  $t = 8$  s, a vertically long cluster (relative size  $S_1 = 0.49$ ) is lifted, which is the signature of the percolation transition. At  $t = 15$  s, the majority of particles are in the largest cluster ( $S_1 = 0.79$ ). At  $t = 120$  s, the largest cluster ( $S_1 = 0.97$ ) becomes compact and rigid, retaining its in-container shape.

**Supplementary Video 3: Pouring particles to create a disentangled state in the DEM simulation.** A total of 4000 disentangled C-particles ( $\theta = 20^\circ$ ) are randomly poured into the conical container under gravity.

**Supplementary Video 4: Entanglement process in the DEM simulation.** C-particles ( $\theta = 20^\circ$ ) are entangling in a container that vertically oscillates with a frequency of 20 Hz and an amplitude of  $0.172D$ . The less entangled state during 2–8 s of the video corresponds to  $t = 0$ –32 s in the experiment. The well-entangled state during 9–16 s of the video corresponds to  $t = 370$ –408 s in the experiment.

**Supplementary Video 5: Lifting clusters near the percolation transition in the DEM simulation.** After being vibrated for  $t = 6$  s, C-particles ( $\theta = 46^\circ$ ) form two large clusters with relative sizes  $S_1 = 0.42$  and  $S_2 = 0.31$ , along with many smaller clusters. The two large clusters are vertically long with comparable sizes, which are two signatures of the percolation transition.

**Supplementary Video 6: Lifting cluster after a long vibration in the DEM simulation.** After being vibrated for  $t = 818$  s, C-particles with  $\theta = 46^\circ$  have well passed the percolation threshold and form a rigid giant cluster with a relative size of  $S_1 = 0.98$  that retains its in-container shape. The other clusters are very small.

**Supplementary Video 7: Stochastic cluster breakage for C-particles with large opening angle  $\theta$  in the DEM simulation.** When the opening angle is relatively large ( $\theta = 138^\circ$ ), the lifted large cluster may break (first three trials as examples) or not break (last three trials as examples). All six trials have the same vibration duration of  $t = 82$  s.

- 
- [S1] P. van Mieghem, *Graph Spectra for Complex Networks* (Cambridge University Press, Cambridge, 2010).
  - [S2] C. P. Dettmann and G. Knight, Symmetric motifs in random geometric graphs, *Journal of Complex Networks* **6**, 95 (2018).
  - [S3] A. Rai, P. Shinde, and S. Jalan, Network spectra for drug-target identification in complex diseases: New guns against old foes, *Applied Network Science* **3**, 51 (2018).
  - [S4] P. Blackwell, M. Edmondson-Jones, and J. Jordan, Spectra of adjacency matrices of random geometric graphs, Department of Probability and Statistics, University of Sheffield (2006).
  - [S5] A. P. Thompson, H. M. Aktulga, R. Berger, D. S. Bolintineanu, W. M. Brown, P. S. Crozier, P. J. in 't Veld, A. Kohlmeyer, S. G. Moore, T. D. Nguyen, R. Shan, M. J. Stevens, J. Tranchida, C. Trott, and S. J. Plimpton, LAMMPS - a flexible simulation tool for particle-based materials modeling at the atomic, meso, and continuum scales, *Computer Physics Communications* **271**, 108171 (2022).
  - [S6] P. A. Cundall and O. D. L. Strack, A discrete numerical model for granular assemblies, *Géotechnique* **29**, 47 (1979).
  - [S7] F. da Cruz, S. Emam, M. Prochnow, J.-N. Roux, and F. Chevoir, Rheophysics of dense granular materials: Discrete simulation of plane shear flows, *Physical Review E* **72**, 021309 (2005).
  - [S8] D. Liu and D. L. Henann, Size-dependence of the flow threshold in dense granular materials, *Soft Matter* **14**, 5294 (2018).
  - [S9] S. Kim and K. Kamrin, Power-Law Scaling in Granular Rheology across Flow Geometries, *Physical Review Letters* **125**, 088002 (2020).
  - [S10] L. E. Silbert, D. Ertas, G. S. Grest, T. C. Halsey, D. Levine, and S. J. Plimpton, Granular flow down an inclined plane: Bagnold scaling and rheology, *Physical Review E* **64**, 051302 (2001).
  - [S11] J. Gaume, G. Chambon, and M. Naaïm, Quasistatic to inertial transition in granular materials and the role of fluctuations, *Physical Review E* **84**, 051304 (2011).

| $N$    | $p_1$             | $p_2$             | $p_3$             |
|--------|-------------------|-------------------|-------------------|
| 500    | $1.025 \pm 0.002$ | $0.103 \pm 0.002$ | $1.455 \pm 0.006$ |
| 4000   | $1.007 \pm 0.001$ | $0.052 \pm 0.001$ | $1.394 \pm 0.007$ |
| 32000  | $1.005 \pm 0.003$ | $0.024 \pm 0.003$ | $1.40 \pm 0.04$   |
| 512000 | $1.004 \pm 0.004$ | $0.008 \pm 0.003$ | $1.46 \pm 0.12$   |

Supplementary Table S2: Fitting parameters  $p_1$ ,  $p_2$ , and  $p_3$  for the fitting curve  $\eta = p_1\langle k \rangle + p_2\langle k \rangle^{p_3}$  in Fig. 4a about the finite-size effects in the ring CP model.

| $\theta$ | Vibration time, $t$ (sec) |    |    |    |    |    |    |    |    |    |    |    |    |     |
|----------|---------------------------|----|----|----|----|----|----|----|----|----|----|----|----|-----|
|          | 0                         | 1  | 2  | 3  | 4  | 6  | 8  | 10 | 15 | 20 | 30 | 40 | 60 | 120 |
| 25°      | 7                         |    | 9  |    | 15 | 17 | 20 | 20 | 15 | 10 | 10 | 7  | 7  | 4   |
| 35°      | 6                         |    | 10 |    | 10 | 15 | 14 | 8  | 4  |    | 4  |    | 4  |     |
| 45°      | 8                         | 9  | 9  | 12 | 12 | 12 | 8  | 7  |    | 6  | 6  |    | 6  |     |
| 55°      | 8                         | 8  | 10 | 10 | 8  | 5  |    | 4  |    | 4  |    |    | 4  |     |
| 70°      | 10                        | 10 | 10 | 8  |    | 5  |    | 5  |    | 4  |    |    | 4  |     |
| 90°      | 11                        | 13 | 13 | 11 | 7  | 7  |    | 5  |    | 4  |    |    | 4  |     |
| 110°     | 4                         | 4  | 4  |    | 4  | 6  |    | 7  |    | 6  |    |    | 5  |     |

Supplementary Table S3: Number of trials in the experiments for various opening angles  $\theta$  used in Fig. 1e,h and Extended Data Fig. 1b,c.

| $\theta$         | 70° | 90° | 110° | 115° | 120° | 125° | 130° | 135° |
|------------------|-----|-----|------|------|------|------|------|------|
| Number of trials | 4   | 4   | 6    | 11   | 11   | 7    | 3    | 3    |

Supplementary Table S4: Number of trials in the experiments for various opening angles  $\theta$  at  $t = 60$  sec used in Extended Data Fig. 1f.

| $t$ (sec)              | 0 | 2 | 4 | 6 | 8 | 10 | 15 | 20 | 30 | 40 | 60 |
|------------------------|---|---|---|---|---|----|----|----|----|----|----|
| Number of measurements | 1 | 2 | 8 | 9 | 9 | 9  | 9  | 2  | 2  | 2  | 2  |

Supplementary Table S5: Number of experimental trials in measuring the vertical length  $L_z$  used in Extended Data Fig. 5a. The opening angle  $\theta = 25^\circ$ .

| $\theta$ | Vibration time, $t$ (sec) |      |    |    |     |     |     |     |     |    |    |    |    |    |    |    |    |     |     |     |     |
|----------|---------------------------|------|----|----|-----|-----|-----|-----|-----|----|----|----|----|----|----|----|----|-----|-----|-----|-----|
|          | 0                         | 0.51 | 1  | 2  | 3.1 | 4.1 | 5.1 | 6.1 | 8.2 | 10 | 12 | 16 | 20 | 25 | 37 | 53 | 82 | 164 | 245 | 327 | 409 |
| 20°      | 4                         |      |    | 4  |     | 5   |     |     | 7   |    | 20 | 20 | 20 | 20 | 15 | 15 | 15 | 10  | 10  | 10  | 10  |
| 33°      | 4                         |      |    | 5  |     | 5   |     |     | 15  | 15 | 15 | 15 | 20 | 15 | 12 | 9  | 9  | 7   | 7   | 7   | 7   |
| 46°      | 5                         |      |    | 10 |     | 20  | 20  | 20  | 15  |    | 15 | 15 |    | 15 | 15 | 7  | 7  | 7   | 7   | 7   | 7   |
| 59°      | 5                         | 10   | 15 | 15 | 15  | 15  |     |     | 15  |    | 15 | 15 |    | 15 | 9  | 7  | 7  | 7   | 7   | 7   | 7   |
| 72°      | 10                        | 20   | 20 | 20 |     | 20  |     |     | 20  |    |    | 20 |    | 20 | 16 | 7  | 7  | 7   | 7   | 7   | 7   |
| 98°      | 10                        | 15   |    | 15 |     | 15  |     |     | 15  |    |    | 15 |    | 15 |    | 15 | 15 | 15  | 7   | 7   | 7   |
| 112°     | 5                         |      |    | 7  |     |     |     |     | 10  |    |    | 15 |    | 15 | 15 | 15 | 15 | 15  | 10  | 10  | 10  |
| 125°     | 5                         |      |    |    |     |     |     |     | 15  |    |    | 16 |    | 20 | 20 | 20 | 19 | 15  | 10  | 10  | 10  |
| 138°     | 3                         |      |    |    |     |     |     |     | 5   |    |    | 5  |    | 10 | 10 | 10 | 15 | 15  | 15  | 15  | 15  |
| 151°     |                           |      |    |    |     |     |     |     | 5   |    |    | 5  |    | 5  |    | 5  | 5  | 5   | 5   | 5   | 10  |

Supplementary Table S6: Number of trials in DEM simulations for various opening angles  $\theta$  used in Fig. 1–3, Extended Data Fig. 1–6, 8, 9. The number of particles  $N = 4000$  in each system.

| <i>N</i> | Vibration time, <i>t</i> (sec) |   |     |     |    |    |    |    |    |    |    |     |     |     |     |     |     |      |      |      |
|----------|--------------------------------|---|-----|-----|----|----|----|----|----|----|----|-----|-----|-----|-----|-----|-----|------|------|------|
|          | 0                              | 2 | 4.1 | 8.2 | 12 | 16 | 20 | 25 | 37 | 53 | 82 | 164 | 245 | 327 | 409 | 572 | 818 | 1227 | 1635 | 2044 |
| 500      | 10                             |   |     | 27  |    | 27 |    | 32 | 32 | 32 | 32 | 32  | 32  | 20  | 20  | 10  | 10  | 10   | 10   | 10   |
| 1400     | 7                              |   |     | 25  |    | 25 | 25 | 25 | 25 | 25 | 23 | 15  | 15  | 15  | 15  | 10  | 6   |      |      |      |
| 4000     | 4                              | 4 | 5   | 7   | 20 | 20 | 20 | 20 | 15 | 15 | 15 | 10  | 10  | 10  | 10  | 5   | 5   |      |      |      |

Supplementary Table S7: Number of trials in DEM simulations for different total number of particles *N* used in Fig. 4e,f and Extended Data Fig. 7e,f. The opening angle  $\theta = 20^\circ$ .

| $\eta$ | Ring | Sphere |
|--------|------|--------|
| 0.1    | 2000 | 2000   |
| 0.5    | 2000 | 2000   |
| 0.9    | 2000 | 2000   |
| 1.3    | 2000 | 2000   |
| 1.7    | 2000 | 2000   |
| 1.8    |      | 2000   |
| 1.9    | 2000 | 2000   |
| 1.95   |      | 2000   |
| 2      | 2000 | 2000   |
| 2.08   | 2000 | 2000   |
| 2.16   | 2000 | 2000   |
| 2.24   | 2000 | 2000   |
| 2.32   | 2000 | 2000   |
| 2.4    | 2000 | 2000   |
| 2.48   | 2000 | 2000   |
| 2.56   | 2000 | 2000   |
| 2.64   | 2000 | 2000   |
| 2.72   | 2000 | 2000   |
| 2.8    | 2000 | 2000   |
| 2.9    | 2000 | 2000   |
| 3      | 2000 | 2000   |
| 3.1    | 2000 | 2000   |
| 3.2    | 2000 | 2000   |
| 3.3    | 2000 | 2000   |
| 3.4    | 2000 | 2000   |
| 3.5    | 2000 | 2000   |
| 3.6    | 2000 | 2000   |
| 3.8    | 2000 | 2000   |
| 4      | 2000 | 2000   |
| 4.2    | 2000 | 2000   |
| 4.4    | 2000 | 2000   |
| 4.6    | 2000 | 2000   |
| 4.8    | 2000 | 2000   |
| 5      | 2000 | 2000   |
| 5.5    | 2000 | 2000   |
| 6      | 2000 | 2000   |
| 6.5    | 2000 | 2000   |
| 7      | 2000 | 2000   |
| 7.5    | 2000 | 2000   |
| 8      | 2000 | 2000   |
| 9      | 2000 | 2000   |
| 10     | 2000 | 2000   |
| 12     | 2000 | 2000   |
| 16     | 2000 | 2000   |
| 22     | 2000 | 2000   |
| 28     | 2000 | 2000   |
| 34     | 2000 | 2000   |

Supplementary Table S8: Number of trials in Monte Carlo simulations of the two CP models (ring and sphere) for various reduced density ( $\eta = n\pi D^3/3$ ), which are used for black curves in Fig. 3a,b,d,e, Extended Data Fig. 4, and Extended Data Fig. 6i,j.  $N = 4000$  in each system.

| $\eta$ | $N = 500$ | $N = 4000$ | $N = 32000$ | $N = 512000$ |
|--------|-----------|------------|-------------|--------------|
| 1      | 2000000   | 250000     | 31250       | 1953         |
| 1.4    | 2000000   | 250000     | 31250       | 1953         |
| 1.8    | 2000000   | 250000     | 31250       | 1953         |
| 1.9    | 2000000   | 250000     | 31250       | 1953         |
| 2      | 2000000   | 250000     | 31250       | 1953         |
| 2.02   |           | 250000     | 3125        | 7813         |
| 2.04   |           | 250000     | 3125        | 7813         |
| 2.06   |           | 250000     | 3125        | 7813         |
| 2.08   |           | 250000     | 3125        | 7813         |
| 2.1    | 12000000  | 1500000    | 187500      | 11719        |
| 2.105  | 12000000  | 1500000    | 187500      | 11719        |
| 2.11   | 12000000  | 1500000    | 187500      | 11719        |
| 2.115  |           | 1500000    | 187500      | 11719        |
| 2.12   |           | 250000     | 3125        |              |
| 2.13   |           |            |             | 7813         |
| 2.14   |           | 250000     | 3125        | 7813         |
| 2.15   |           |            |             | 7813         |
| 2.16   |           | 250000     | 31250       | 7813         |
| 2.17   |           |            | 31250       |              |
| 2.18   |           | 250000     | 31250       |              |
| 2.19   |           |            | 31250       |              |
| 2.2    | 2000000   | 250000     | 31250       | 1953         |
| 2.21   |           |            | 31250       |              |
| 2.22   |           | 250000     |             |              |
| 2.22   |           |            | 31250       |              |
| 2.24   |           | 250000     | 3125        |              |
| 2.25   |           |            |             | 7813         |
| 2.26   |           | 250000     | 3125        |              |
| 2.28   |           | 250000     | 3125        |              |
| 2.3    | 2000000   | 250000     | 31250       | 1953         |
| 2.325  | 2000000   |            |             |              |
| 2.35   | 2000000   |            |             |              |
| 2.375  | 2000000   |            |             |              |
| 2.4    | 2000000   | 250000     | 31250       | 1953         |
| 2.425  | 2000000   |            |             |              |
| 2.45   | 2000000   |            |             |              |
| 2.475  | 2000000   |            |             |              |
| 2.5    | 2000000   | 250000     | 31250       | 1953         |
| 2.6    | 2000000   | 250000     | 31250       | 1953         |
| 2.7    | 2000000   | 250000     | 31250       | 1953         |
| 2.8    | 2000000   | 250000     | 31250       | 1953         |
| 2.9    | 2000000   | 250000     | 31250       | 1953         |
| 3      | 2000000   | 250000     | 31250       | 1953         |
| 3.2    | 2000000   | 250000     | 31250       | 1953         |
| 3.6    | 2000000   | 250000     | 31250       | 1953         |
| 4      | 2000000   | 250000     | 31250       | 1953         |
| 5      | 2000000   | 250000     | 31250       | 1953         |

Supplementary Table S9: Number of trials in Monte Carlo simulations of ring CP model for various reduced density ( $\eta = n\pi D^3/3$ ) and number of particles ( $N$ ), which are used in Fig. 3g, Fig. 4a-d, Extended Data Fig. 6a-h, and Extended Data Fig. 7.
